# Supplementary material for: Self-assembly and non-equilibrium phase coexistence in a binary granular mixture
Source: arXiv:2410.21576 ancillary file (2024-10-28)
Supplement: Supplementary file 1 [file SM.pdf]

# SUPPLEMENTARY MATERIAL
# (Self-assembly and non-equilibrium phase coexistence in a binary granular mixture)

## DETAILS OF THE EXPERIMENTAL PROCEDURE

Here we provide additional details on the experimental setup. We recall that this work has been done with the same setup used in Ref. 1. The reader can also refer to its Methods section and Supplementary Information for details about image processing and acceleration measurements of the plate.

### Horizontal calibration of the setup

The inclination of the plate is adjusted using three levelling feet that support the apparatus. Before each experimental session, we followed a calibration procedure consisting of different steps. First, a preliminary rough adjustment is made using an electronic level (Laserliner). Next, we vibrate a dilute monodisperse system of large grains (with diameters $\sigma_L = 2.5$ mm for steel and $\sigma_L = 4$ mm for polyamide) and analyze the time-averaged density field after a 20-minute data acquisition. The vibration parameters are set to $f = 120$ Hz, $\Gamma = 1.48$ for steel, and $f = 53$ Hz, $\Gamma = 1.87$ for polyamide, chosen to produce gas-like motion in the grains. Steel grains are vibrated on a smooth surface and polyamide grains on a sandblasted one (see the next Section).

For a perfectly calibrated surface, we expect the density field to exhibit mirror symmetry along both the x- and y-axes, although uniformity is not expected due to dissipative effects near the walls. However, following the initial adjustment with the level, the density field consistently shows higher intensity in a particular direction, indicating the influence of gravity. To address this, we fine-tune the levelling feet based on the observed asymmetry and repeat the process to achieve a more symmetric density distribution. As mentioned in the main text, extended experiments may result in some loss of horizontal calibration, but this does not significantly impact the self-assembly process.

## EXPERIMENTAL CALIBRATION OF DRIVING PARAMETERS

In this section, we describe the initial experiments used to calibrate the driving conditions for the longer-term self-assembly runs. In these experiments, we explored the effect of the non-equilibrium parameters without substantially varying the geometrical constraints $\{q, x_S, \phi\}$. We considered two different materials for the grains and for each of them we varied the driving parameters to find good conditions for the self-assembly process. We used both polyamide (PROLABO) and steel (Marteau & Lemarié) beads. Note that in the main text, only the polyamide results are reported. For polyamide beads we have diameters $\sigma_S = 2$ mm, $\sigma_L = 4$ mm; the density is $\rho = 1.14$ g/cm$^3$. For steel beads $\sigma_S = 1.2$ mm, $\sigma_L = 2.5$ mm, $\rho = 7.85$ g/cm$^3$. and $L = 10$ cm.

We first discuss the results of two different experiments, one with steel beads and one with polyamide beads; both of them were performed with sinusoidal vibrations. We recall here that the bottom surface used with polyamide grains has been sandblasted to increase its roughness. This is not possible with steel grains, which are harder and tend to smooth out the rough surface after repeated collisions, a problem that is particularly relevant in our case since we need to perform very long experiments. With steel beads we use a smooth surface as done in [1].

An important difference between the two considered cases is the range of driving parameters $\{\Gamma, f\}$ we can impose on the system. As we found in a previous study [1], good driving conditions for granular self-assembly must be such that the system can effectively explore the spatial configurations in the horizontal plane while remaining relatively confined in the vertical direction to prevent small particles from jumping on top of each other and thus altering the effective 2D area fraction of the system. Hence, for both systems, we must find the combinations of $\Gamma$ and $f$ for which these requirements are satisfied. The key advantage of using a sandblasted bottom plate is that the presence of surface asperities significantly enhances the $z$-to-$xy$ energy in plate-grain collisions [2, 3]. Thus, with polyamide beads on a rough surface, we are able to enhance the horizontal mobility using stronger vibrations that, in the case of steel beads on a smooth surface, would also imply a considerable exploration of the vertical direction in the grain dynamics. Quantitatively, for polyamide beads, we find an optimal driving condition for $\Gamma = \Gamma_p = 1.79$ at $f = f_p = 53$ Hz while for steel beads, we use $\Gamma = \Gamma_s = 1.28$ and $f = f_s = 120$ Hz. It is important to note that, although these driving conditions only differ by a factor $\Gamma_p/\Gamma_s = 1.40$ in acceleration, they correspond to displacement amplitudes of $A_p = g\Gamma_p/f_p^2 = 158\mu$m and $A_s = g\Gamma_s/f_s^2 = 22\mu$m for polyamide and steel particles respectively. This leads, in

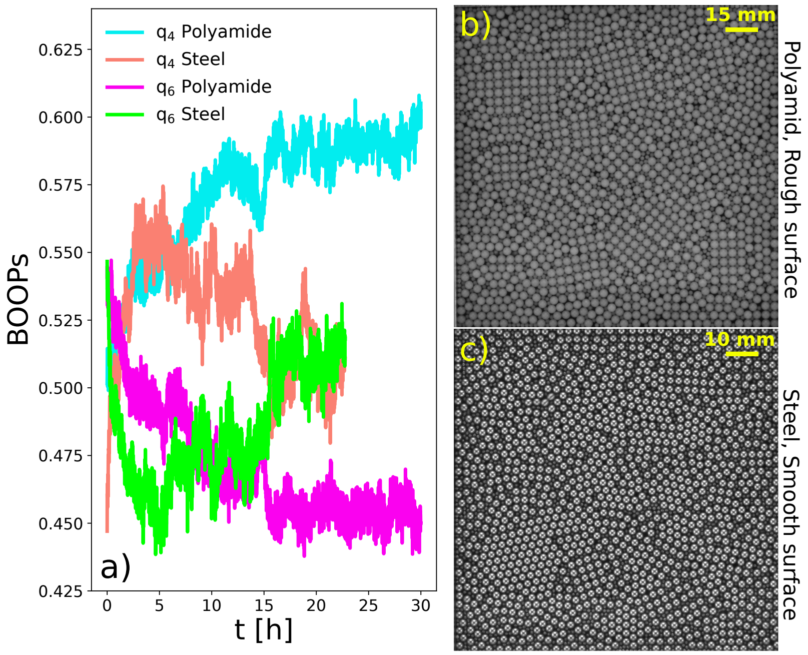


FIG. 1. a) Time evolution of $q_4$ and $q_6$ obtained with polyamide and steel beads under sinusoidal vibrations. For polyamide grains $q = 0.5$, $x_S = 0.5$, $\phi = 0.851$, $\Gamma = 1.79$, $f = 53$ Hz and the bottom surface is sandblasted. For steel grains $q = 0.48$, $x_S = 0.52$, $\phi = 0.855$, $\Gamma = 1.28$, $f = 120$ Hz and the bottom surface is smooth. b) Final configuration obtained with polyamide beads with several S1 patches widespread all over the system. c) Final configuration obtained with steel beads with large hexagonal clusters and a few small S1 domains.

turn, to a change in the shaking energy of a factor $A_p^2 f_p^2/(A_s^2 f_s^2) = 10$. Finally, the values of $\sigma_S$ and $\sigma_L$ for polyamide and steel beads are different but the imposed geometrical constraints $\{q, x_S, \phi\}$ are approximately the same for the two experiments (see the caption of Fig. 1). In Fig. 1a-c, we plot the BOOPs (see the definition in the main text) as a function of time and provide a direct visualization of the final configurations of the system. The evolution of the BOOPs is qualitatively similar in the two experiments for the first 5 hours, exhibiting an increase of $q_4$ and a decrease of $q_6$. During this time, we observed the self-assembly of S1 domains in different regions of the system. After that, steel beads show an arrest of the S1 formation coinciding with the growth of hexagonal clusters of large particles which result in being particularly stable and hard to melt. For polyamide grains, we found instead a further increase of $q_4$ which is related to agglomeration and growth of the S1 patches. Here, no significant formation of hexagonal domains is observed. It can be concluded that the system with steel beads driven on the smooth surface at $\{\Gamma_s, f_s\}$ is more prone to crystallization into hexagonal crystals than the one with polyamide beads driven on the rough surface at $\{\Gamma_p, f_p\}$. Here we try to explain this idea in terms of energy transfer mechanisms. We hypothesise that, in the system with steel beads, the energy is injected in the horizontal plane mainly by off-planar collisions and these are favoured when considering particles of different sizes. On the other hand, particles of identical size will have much less occasion of undergoing off-planar collisions with a relevant energy transfer between vertical and horizontal directions. Following this idea, it is reasonable to expect hexagonal clusters of grains of the same size to be particularly stable. As suggested by previous experimental studies [1], using granular mixtures with a higher fraction of small particles results in more homogeneous horizontal fluidization of the system. However, in our case, we cannot adopt this solution since we are interested in keeping $x_S \simeq 0.5$, i.e. close to the value that leads to S1 formation in the equilibrium reference system.

For the polyamide case, we can use a rough bottom surface, along with stronger vibrations, which strongly changes the situation. Indeed, grain-plate collisions alone are capable of transferring considerable energy from $z$ to $xy$, regardless of the local structure of the system. We conclude that a more efficient local injection of energy in the horizontal plane helps the system to remain homogeneously fluidized. Further experiments would be needed to definitively confirm this picture, but this goes beyond this study.

Experimentation with the shape of the driving signal showed that one way of improving the mobility of the steel beads was to use sawtooth driving signals instead of sinusoidal ones. Sawtooth vibrations are obtained imposing an acceleration $a_z(t) = g\Gamma[(ft \bmod 1) - 1/2]$ so they are still parametrized by the frequency $f$ and the amplitude $\Gamma$. We

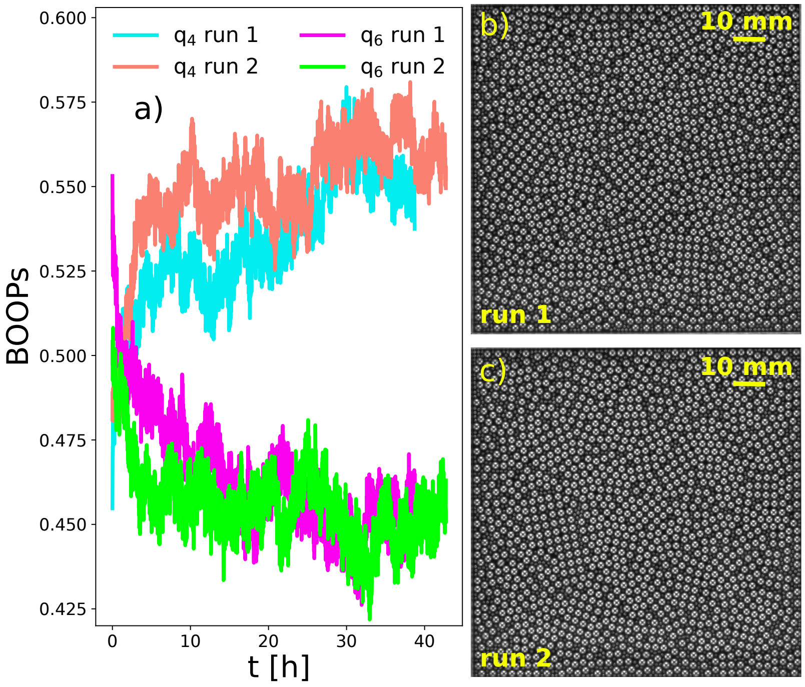


FIG. 2. Results from two independent experimental runs with steel beads on a sandblasted surface under sawtooth vibrations. For both experiments $q = 0.48$, $x_S = 0.52$, $\phi = 0.856$, $\Gamma = 2.13$, $f = 110$ Hz. a) Time evolution of $q_4$ and $q_6$. b) Final configurations with S1 patches and no relevant presence of hexagonal clusters.

found that with this type of driving it was possible to increase the strength of the vibrations without triggering a relevant exploration of the vertical direction in the grain dynamics. This resulted in a stronger and more homogeneous horizontal fluidization of the system (but still weaker than the one obtained with polyamide beads on a rough surface). In Fig. 2, we show the results obtained with steel beads on a smooth surface under sawtooth vibrations with $\Gamma = 2.13$ and $f = 110$ Hz. We point out that in this case the S1 patches are more stable and the results are reproducible (we show data coming from two independent runs). However, when comparing the final configurations obtained with steel grains on a smooth surface and those obtained with polyamide grains on a rough surface, we always found larger and more widespread S1 domains in the latter case (compare for example Fig. 1b and Fig. 2b or 2c ). Hence, in the main text, we only considered results obtained in the optimal experimental conditions we found for S1 self-assembly thus using polyamide beads on a rough surface under sinusoidal vibrations.

## CALIBRATION OF DIRECT PHASE COEXISTENCE SIMULATIONS

The direct coexistence method involves directly bringing two phases (performed as initial conditions) into contact around their respective coexistence densities and allowing the system to reach a steady state to measure its equilibrium coexistence properties. While this procedure is straightforward for fluid-fluid coexistence, additional care is required when at least one of the phases is a crystal. Specifically, it is important to ensure that the equilibrated crystal does not develop additional strain in the direction perpendicular to the interface due to boundary condition effects [4, 5]. Indeed, if the interface is perpendicular to the $x$ axis, and the length of the simulation box in the $y$-direction is fixed, the crystal structure along the $y$ axis cannot relax and notably, its lattice spacing will not change with time. Therefore, it is necessary to run multiple simulations with initial crystals of varying initial lattice spacing $a_y$, and identify the final steady system in which $a_y = a_x$. Here, $a_x$ is the measured lattice spacing, which can relax over time due to the fluid interface. This approach can be seen as a generalization of the stress-tensor-based method of Ref. 5. Although measurements of the crystal lattice spacing are somewhat more cumbersome (and likely less statistically accurate) than measuring the stress tensor, for non-equilibrium systems it has the advantage of avoiding the need for a robust method for measuring non-equilibrium stresses.

In DEM simulations, we start with a unique slab of S1 crystal and then let melt it until stable coexistence between

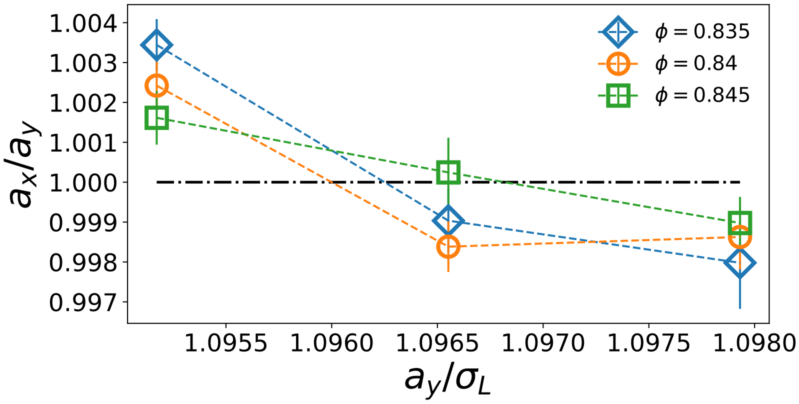


FIG. 3. Averaged $a_x/a_y$ as a function of $a_y$ for different area fractions in DEM simulations. Other fixed parameters are: $N = 3600$, $q = 0.476$, $x_S = 0.5$, $\Gamma = 4.4$ and $f = 350$ Hz.

the liquid and the crystalline slab is reached. We perform simulations with a fixed number of grains without varying the number of columns and rows in the initial crystal. Then, we can tune $L_x$ and $L_y$ to satisfy the imposed global area fraction $\phi$. Here, the initial lattice spacing is fixed by $L_y$ since we start with an S1 domain that occupies all the space in the y-direction. Once the system has reached a steady state, we can measure the average ratio $a_x/a_y$ in the remaining crystal. We repeat this procedure for different $L_y$ and $\phi$ until finding the $L_y$ where $a_y/a_x = 1$, such that the crystal phase is undeformed. This process is repeated for different area fractions. In Fig. 3, we show that around $L_y = 31.8\sigma$ we always satisfy this requirement having $a_y/a_x = 1$ with a maximum error lower than 0.004. We then kept $L_y = 31.8\sigma$ fixed for all the simulations discussed in the paper.

For EDMD, we use the following protocol. We run direct coexistence simulations for a sufficient duration to reach a steady state. A typical snapshot is shown in Fig. 4a. We directly measure the average lattice spacing in both the $x$ and $y$ directions, $a_x$ and $a_y$, in real space, as represented by the grey segments in Fig. 4a. The average lattice spacing can also be determined from the positions of the Bragg peaks in the structure factor. We verify that the final measured averaged $a_y$ is approximately equal to the value imposed initially (i.e. the number of layers or the orientation of the crystal did not chance). We perform these measurements for various systems at the same global area fraction but with different initial $a_y$. This procedure results in Fig. 4c, showing the measured averaged $a_x$ as a function of $a_y$. The unstrained crystal corresponds to the crystal at which $a_y/a_x = 1$ which is found through a linear fit of $a_y/a_x$ as a function of $a_y$.

These simulations also allow us to obtain local area fractions, $\phi(x)$ through averaging multiple snapshots. This averaged profile is given in Fig. 4b. The average densities of the liquid and solid phases are determined by finding the mean values of the two plateaus in $\phi(x)$. Hence, for each simulation at a given $a_y$, the coexistence densities can be obtained, as seen in Fig. 4d. The correct ones correspond to those of the unstrained crystal, $a_y$ is such that $a_y/a_x = 1$ (stars), which was obtained in Fig. 4c. This method is then performed for different physical parameters to obtain the phase diagrams presented in the main text.

## HYBRID EVENT-DRIVEN/TIME-STEPPED MOLECULAR DYNAMICS

Since the potential of hard-disk particles is discontinuous, usual time-stepped molecular dynamics methods are not suitable for simulations of such systems. Instead, we use event-driven methods [6] where the time before the collision of two particles $i$ and $j$ denoted $t_{ij}^{col}$ can be analytically computed:

$$|\boldsymbol{r}_i(t_{ij}^{col}) + \boldsymbol{r}_j(t_{ij}^{col})| = \frac{\sigma_i + \sigma_j}{2}, \qquad (1)$$

with $\boldsymbol{r}_i(t)$ the position of particle $i$ at time $t$. For particles free flying or undergoing constant viscous drag, $t_{col}^{ij}$ can be found exactly from the initial velocities and positions of the particles. The viscous friction due to the thermostat is applied continuously on the velocities in between events. This exponential decay of the velocity leads to the following

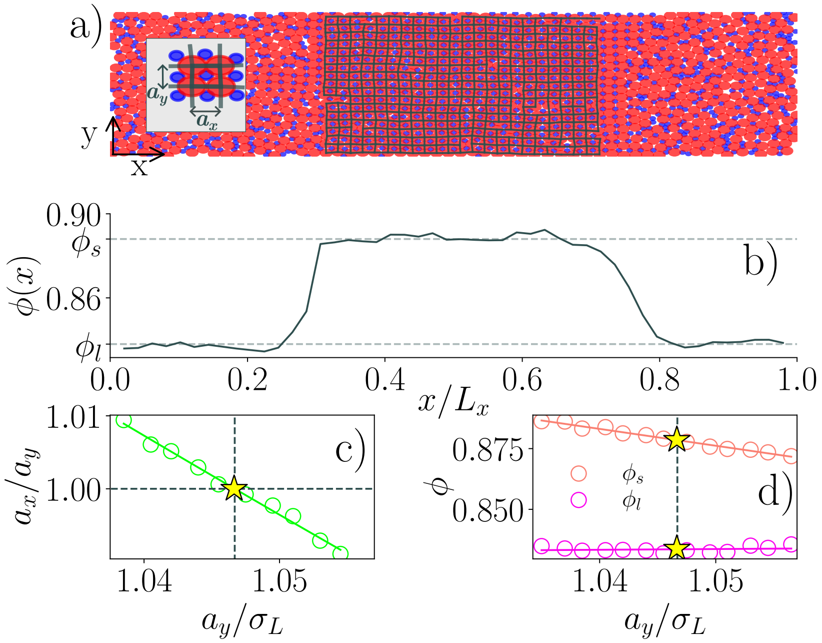


FIG. 4. Protocol used in EDMD simulations to obtain the solid and liquid coexistence densities. a) A typical coexistence configuration in its steady state. The segments in grey in the middle of the box show the numerically found values of the local lattice spacing (as shown in the Inset). $N = 1944$ b) The corresponding local area fraction obtained from an average of 150 (shifted) snapshots of the steady state pictured in panel a). c) Values of the average $a_y/a_x$ as a function of the initial (and because of stability, final) $a_y$. Each point corresponds to a different simulation with the same global area fraction but different initial $a_y$. The measurements are taken in the steady state and averaged over 10 configurations. The point at which $a_y/a_x = 1$ corresponds to an unstrained crystal. This informs us about the correct $a_y$ to impose at the beginning so that we can measure the correct coexistence densities. d) The measured liquid and solid densities (as seen in b)) for different initial $a_y$. The correct densities are the ones for which $a_y$ is equal to the one chosen from c). $N = 9600$, $q = 0.476$, $x_s = 0.5$ and $\alpha = 0.97$.

collision time between two collisions:

$$t_{ij}^{col} = -\log\left(1 - \gamma\, \delta t_{ij}\right)/\gamma, \tag{2}$$

with:

$$\delta t_{ij} = \frac{-b - \sqrt{b^2 - \boldsymbol{v}_{ij}^2\left(\boldsymbol{r}_{ij}^2 - (\sigma_i \sigma_j)^2\right)}}{\boldsymbol{v}_{ij}^2} \tag{3}$$

where $b = \boldsymbol{r}_{ij} \cdot \boldsymbol{v}_{ij}$ and $\boldsymbol{r}_{ij}$ and $\boldsymbol{v}_{ij}$ are respectively the relative position and velocity of particles $i$ and $j$ at the moment the subsequent collision time is computed.

The thermostat is modelled by a time-driven instantaneous change of the velocity of every particle each $\Delta t_{\text{noise}}$ (in between the particle-particle collisions) according to:

$$\boldsymbol{v}_i' = \boldsymbol{v}_i + \sqrt{2\gamma T_b \Delta t_{\text{noise}}/m_i}\,\boldsymbol{\eta}(t) \tag{4}$$

with $\boldsymbol{\eta}(t)$ a Gaussian white noise with zero average and unit variance. After the application of this noise, every collision time must be recomputed.

The fluctuation-dissipation theorem is respected (at equilibrium) for reasonable values of $\Delta t_{\text{noise}}$ because of the continuous nature of the damping [7]. We nonetheless chose $\Delta t_{\text{noise}} \ll \tau_f$, with $\tau_f$ the mean free time.

[1] A. Plati, R. Maire, E. Fayen, F. Boulogne, F. Restagno, F. Smallenburg, and G. Foffi, Nat. Phys. **20**, 465 (2024).
[2] P. M. Reis, R. A. Ingale, and M. D. Shattuck, Phys. Rev. E **75**, 051311 (2007).
[3] G. Gradenigo, A. Sarracino, D. Villamaina, and A. Puglisi, Europhys. Lett. **96**, 14004 (2011).

[4] J. R. Espinosa, E. Sanz, C. Valeriani, and C. Vega, J. Chem. Phys. **139** (2013).
[5] F. Smallenburg, G. Del Monte, M. de Jager, and L. Filion, J. Chem. Phys. **160** (2024).
[6] F. Smallenburg, Eur. Phys. J. E **45**, 22 (2022).
[7] L. Ma, X. Li, and C. Liu, Commun. Math. Sci. **15**, 1171 (2017).
